# Supplementary material for: Crystal structure, stability and optoelectronic properties of the organic-inorganic wide bandgap perovskite CH3NH3BaI3: Candidate for transparent conductor applications
Source: arXiv:1604.08003 source file (2016-09-28)
Supplement: Supplementary file 1 [file Supplementary.pdf]

# Supplementary Material

## Crystal structure, stability and optoelectronic properties of the organic-inorganic wide bandgap perovskite $CH_3NH_3BaI_3$: Candidate for transparent conductor applications

*Akash Kumar[1+], Jiban Kangsabanik[2+], Vikram [2+], Aftab Alam[2], K.R. Balasubramaniam[1]*

*[1] Department of Energy Science and Engineering, IIT Bombay, Mumbai, Maharashtra, 400076, India*

*[2] Department of Physics, IIT Bombay, Mumbai, Maharashtra, 400076, India*

**PACS number -81.15.-z, 81.10.Dn, 31.15.E-, 61.50.Ah, 61.10.Nz, 42.70.Qs, 71.20.-b**

([+]These three authors have contributed equally to this work)

Here, we provide further experimental and numerical data and related discussions to strengthen our message in the manuscript.

### Section 1 : Synthesis technique

Solution processing was chosen as our preferred synthesis technique over others, such as vapor deposition or vapor assisted solution processing, owing to the ease of obtaining the thin film at low temperatures. The first step in the processing of thin films *via* solution processing was to determine a common solvent for both the organic and inorganic precursors, $CH_3NH_3I$ and $BaI_2$. The organic precursor has been found to be easily dissolved in various non-polar solvents, e.g. DMF (Dimethyl formamide), GBL (Gamma Butyrolactone), DMSO (Dimethyl sulphoxide) etc. So, we performed the solubility check of $BaI_2$ in these solvents. Our observations suggest that DMF is a better solvent in comparison to GBL and DMSO.

**Synthesis of methyl-ammonium iodide-** 32.2 ml. $CH_3NH_2$ (in 40 % $CH_3OH$) and 30 ml. HI (in 57 % $H_2O$) was mixed and maintained at 0 °C for 2 hours. The solution was then kept in rotary evaporator at 50 °C and precipitated. Obtained precipitated powder was washed in di-ethyl ether for 30 minutes for 3 times. Final product was recrystallized in di-ethyl ether and ethanol. The powder, thereafter, was kept in vacuum furnace for 24 hours at 60 °C to synthesize methyl-ammonium iodide. Since the constituent chemicals (methylamine and hydriodic acid) starts degrading at very low temperature (-6 °C and -35.6 °C respectively), it is made sure that any of the synthesis step does not denaturizes the final desired product by any high temperature step during the synthesis process.

XRD analysis of the $CH_3NH_3BaI_3$ thin film samples synthesized after 12, 24, 48 and 96 h of the formation of the solution was done. As can be seen in the Fig. S1.1 no peaks were observed suggesting that crystallization has not been initiated even upto 96 h.

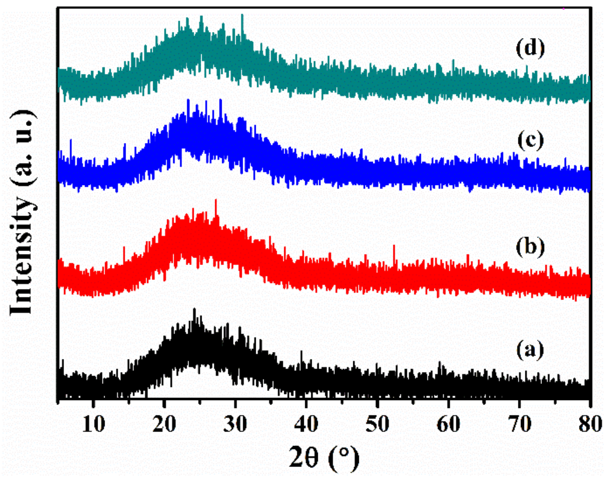


**Fig. S1.1** (Color online) XRD patterns of the $CH_3NH_3BaI_3$ films made after holding the precursor solution under ambient condition for different durations; (a) 12 h, (b) 24 h, (c) 48 h and (d) 96 h. No crystalline peaks are observed in any of the samples.

**Section 2 : Simulated XRD pattern:** Based on the atom positions, Powder XRD was simulated using CrystalMaker program. Fig. S2.1 shows such a simulated powder XRD pattern of $CH_3NH_3BaI_3$. It should be noted that the peak intensity for the peaks (00*l*) {*l* = 2, 6, 8, 10} is very less in comparison to (004) peak, similar to the peak intensity trend as observed in our experimental XRD pattern.

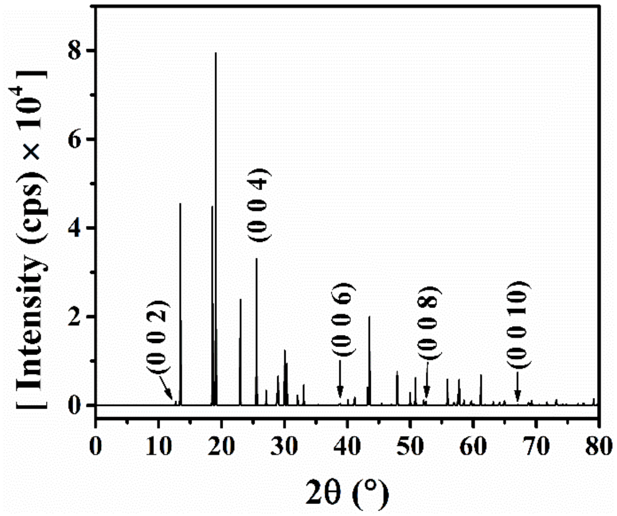


**Fig. S2.1** Simulated powder XRD of $CH_3NH_3BaI_3$ indicating peak positions of (00*l*) {*l*=2, 4, 6, 8, 10} peaks.

**Section 3 : Computational details:-**

The *ab initio* calculations were done using Density functional theory (DFT) using plane wave basis set as implemented in VASP. We used Projector Augmented Wave (PAW) pseudo potentials with PBE exchange correlation functional. C 2s2/2p2, H 1s1, N 2s2/2p3, Ba 5s2/5p6/6s2, I 5s2/5p5, La 5p6/5d1/6s2 electrons were treated as valence electrons. The Brillouin zone sampling was done by using 3x3x2 K-point mesh for relaxation and 12x12x8 for static calculations of MABaI3.

Lattice dynamics calculations were done to estimate elastic properties from the Hessian matrix obtained using finite difference approach. 3x3x2 K point mesh

and a step size of 0.015 Å was used for the displacement of atoms for this calculation.

Defect formation energies are calculated using a 2x2x2 (384 atoms) supercell using a gamma point only reciprocal mesh.

Calculations for various concentration of La doping were performed by taking 2x2x2 (384 atoms), 2x2x1 (192 atoms) and 2x1x1 (96 atoms) supercells and replacing one Ba atom with La to achieve 3.125%, 6.25% and 12.5 % La-doping respectively.

## Section 4 : Structural Details and Formation energy:-

**Table S4.1** Relaxed atomic positions of constituent atoms for the $CH_3NH_3I$ structure in Cartesian co-ordinates.

| **Atomic Coordinates (Å)** | | | |
|---|---|---|---|
| **C** | 2.521572217 | 4.962486022 | 6.568424854 |
| **C** | 5.544359153 | 2.271954213 | 1.672848464 |
| **N** | 2.382787933 | 0.214886557 | 5.752991020 |
| **N** | -0.085942834 | 3.317293956 | 2.729189786 |
| **H** | 5.029832644 | 0.366341039 | 4.029087970 |
| **H** | 2.241098974 | 5.085058209 | 7.615501732 |
| **H** | 3.157603690 | 4.125285017 | 6.284372367 |
| **H** | 0.747836716 | 1.616537805 | 1.781264287 |
| **H** | 5.573814859 | 2.764979456 | 0.694199729 |
| **H** | 4.621724371 | 1.688206244 | 1.773831081 |
| **H** | 1.836182448 | 1.056388940 | 6.009550352 |
| **H** | 5.332768839 | 0.669455147 | 4.650057723 |
| **H** | 2.652958292 | 0.119741680 | 4.761484579 |
| **H** | 4.733442013 | 3.933204257 | 2.659265063 |
| **H** | 0.762388337 | 3.929092744 | 2.610043996 |
| **H** | -0.045837884 | 2.939293385 | 3.696846786 |

| | | | |
|---|---|---|---|
| **I** | 2.744211763 | 5.267315918 | 2.174906688 |
| **I** | 0.365786419 | 3.113183704 | 6.363689820 |

In order to compare the relative chemical stability, we have calculated the formation energy of four perovskites ($CH_3NH_3BI_3$ : $B$ = Ba, Pb, Ca, Sr). A complete relaxation was done for the tetragonal structure of all these compounds. The calculation details are same as given in section 3. To estimate the formations energies, one also need the energetics for the parent compounds $CH_3NH_3I$ and $BI_2$ ($B$ = Ba, Pb, Ca, Sr). The H-atom positions in the $CH_3NH_3I$ structure, however, are not known (to the best of our knowledge). As such, a direct relaxation of this structure is not possible. So we did this relaxation in two steps. First, we placed the H atoms in the C-N environment taking initial idea from its position in $CH_3NH_3BaI_3$ and did a selective dynamics relaxation allowing only the H atoms to move. Then using the obtained positions, a full relaxation of the $CH_3NH_3I$ structure was performed. The final positions of all the atoms are shown in Table S4.1.

Formation energy(**ΔE**) of $CH_3NH_3BI_3$ is given by,

$$\Delta \mathbf{E} = \frac{1}{48} \left[ \mathbf{p\ E\ (CH_3NH_3}\boldsymbol{B}\mathbf{I_3)} - \mathbf{q\ E(CH_3NH_3I)} - \mathbf{r\ E(}\boldsymbol{B}\mathbf{I_2)} \right]$$

where E(Y) is the total energy for a unit cell of Y compound. p, q and r are the number of unit cell required to make four formula units of the respective compound.

The formation energies of $CH_3NH_3BI_3$ are given in Table S4.2.

**Table S4.2** Formation energies for Ba, Pb, Ca, and Sr based hybrid perovskites

| B | E ($CH_3NH_3BI_3$) (eV/cell) | E($CH_3NH_3I$) (eV/cell) | E($BI_2$) (eV/cell) | ΔE* (meV/atom) |
|---|---|---|---|---|
| **Ba** | -210.5927 | -82.8837 | -41.3642 | -72.11 |
| **Pb** | -203.7775 | -82.8837 | -8.6427 | -71.65 |
| **Ca** | -208.5929 | -82.8837 | -9.9007 | -67.14 |
| **Sr** | -208.75258 | -82.8837 | -78.157719 | -81.37 |

* *Here negative formation energy means structure is stable.*

We have also calculated the defect formation energy for both La-doped as well as vacancy induced defects using the following formula,

$$\Delta E = E_T(\text{defect};q) - \{E_T(\text{perfect}) + \Sigma\, n_i\mu_i\} + q(E_F+E_{VBM})$$

This formula is more appropriate to quantify the stability of various defects in different charge states (**q**) keeping the experimental perspective in mind.[1,2]

Here **$E_T$(defect;q)** is the total energy of the defect crystal in charge state q, **$E_T$(perfect)** is the total energy of perfect crystal without defect, **$n_i$ and $\mu_i$** are respectively the numbers of atoms and chemical potentials of atom i (=Ba, La & I). **$n_i$** is +ve (-ve ) when atom is added (removed) to the perfect supercell to introduce the defect. The values of **$\mu_i$** depend upon the choice of the reference systems. Here **$\mu_{Ba}$** and **$\mu_I$** is taken from their respective chemical potentials in $BaI_2$ and **$\mu_{La}$** from $LaI_3$. **$E_F$** is the Fermi level measured from the valance band maximum (VBM) and **$E_{VBM}$** is the VBM energy of the defect crystal.

The results for the defect formation energy are shown in Figure 5 (b) of the manuscript.

**Section 5 : DoS of $CH_3NH_3BaI_3$:** Density of states for $CH_3NH_3BaI_3$ can be seen in the Fig. S5.1.

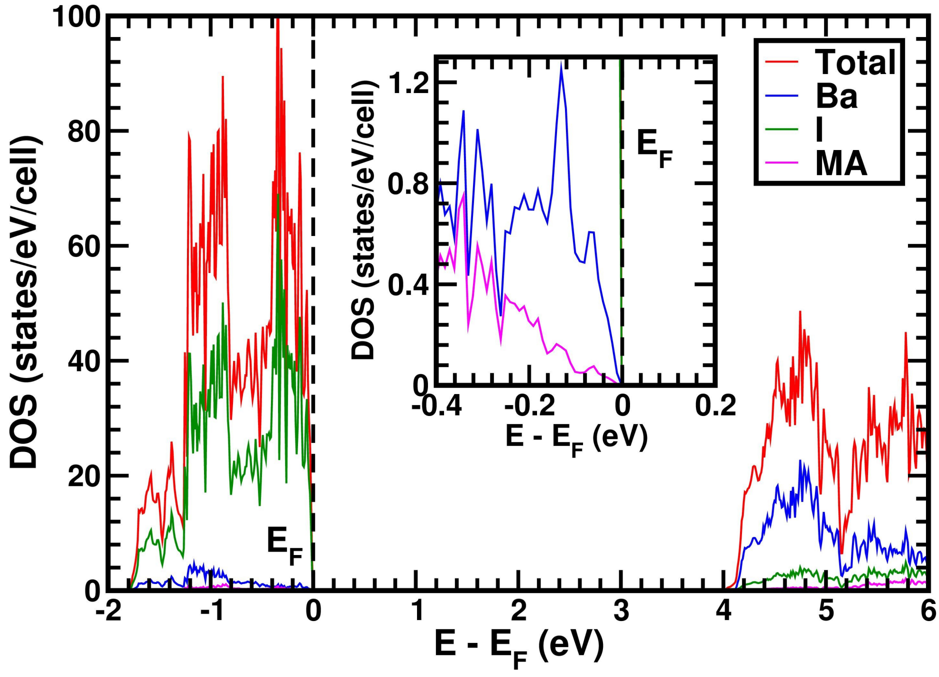


**Fig. S5.1** (Color online) Total and atom projected density of states for $CH_3NH_3BaI_3$. Inset shows a zoomed-in plot near $E_F$. States near/below $E_F$ are majorly dominated by Iodine p-orbitals.

**Section 6 : Bandgap, Charge concentration & Effective mass for $CH_3NH_3(Ba_{1-x}La_x)I_3$:**

Band gap ($\underline{E_g}$), Charge concentration ($\underline{n_C}$), Effective mass (m*) and the ratio ($\underline{n_C}$ /m*) vs. the La doping (x) are shown in the Fig. S6.1. Notice that, although $\underline{n_C}$ increases with increasing La-concentration but m* is not a monotonous function. However, the ratio ($\underline{n_C}$/m*) keeps increasing with x, until 12.5%. This implies the enhancement of conductivity ($\sigma = e^2(\underline{n_C}/m^*)\tau$) with the doping (x) within a non-varying relaxation time (τ) approximation. This is one of the essential requirement for a promising transparent conductor.

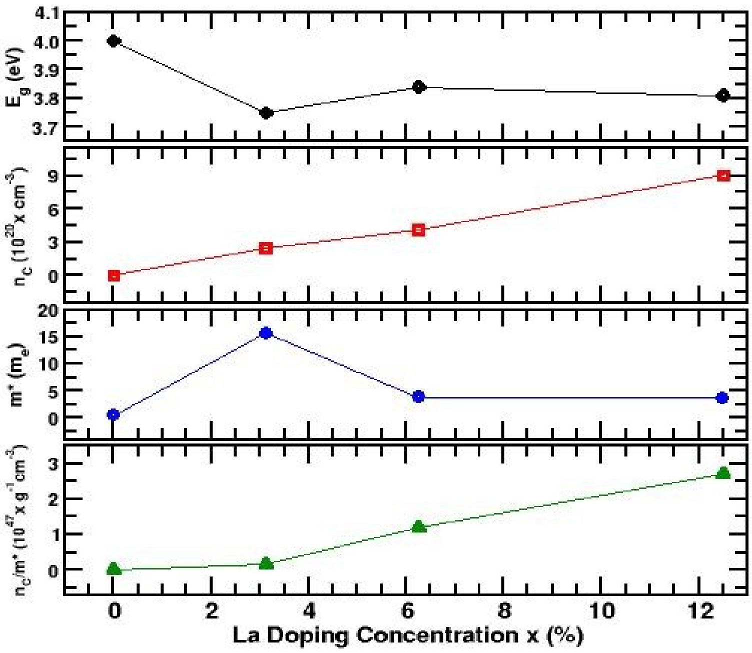


**Fig. S6.1** (Color online) Band gap ($E_g$), Charge concentration ($n_C$) , Effective mass (m*) and the ratio ($n_C$ /m*) as a function of La-doping (x) in $CH_3NH_3(Ba_{1-x}La_x)I_3$.

**References:**


1) Katsuyuki Matsunaga, Tomohito Tanaka, Takahisa Yamamoto, and Yuichi Ikuhara, Phys. Rev. B **68**, 085110

2) David O. Scanlon and Graeme W. Watson, *J. Phys. Chem. Lett.*, ***1*** **(21),** pp 3195–3199 (2010)
